# Supplementary material for: Language-driven Semantic Segmentation
Source: arXiv:2201.03546 source file (2022-04-03)
Supplement: Supplementary file 1 [file appendix.tex]

\section{Appendix}
\label{sec:appendix}
